# Supplementary material for: A single-projection three-dimensional reconstruction algorithm for scanning transmission electron microscopy data
Source: arXiv:2011.07652 source file (2022-02-17)
Supplement: Supplementary file 1 [file Supplementary.pdf]

# Supplementary material

Hamish G. Brown Philipp M. Pelz Shang-Lin Hsu Zimeng Zhang
Ramamoorthy Ramesh Katherine Inzani Evan Sheridan Sinéad M. Griffin
Scott D. Findlay Leslie J. Allen Mary C. Scott Colin Ophus
James Ciston

November 15, 2020

(1)

**Algorithm 1** $\mathcal{S}$-matrix retrieval from a 4D-STEM dataset via gradient descent using an amplitude difference cost function [14, 10]

**Input:**

4D-STEM datasets $I(\Delta f, \mathbf{R}, \mathbf{k})$, with pixel dimensions $(n_{\Delta f}, R_x, R_y, k_x, k_y)$, we denote the total number of scan positions across all defocii $N_{\Delta f, \mathbf{R}_i}$

Lens defoci $\Delta f$ in units of length

Probe positions $\mathbf{R}$ in units of length

Probe forming aperture $k_\alpha$ in units of inverse length

$\mu$, the algorithm "step size"

**Initialize :**

Calculate reconstruction grid dimensions $(M_x/\Delta k_x, M_y/\Delta k_y)$, where $M_i = \text{ceil}(\max(R_i) - \min(R_i))\Delta k_i$ for $i = x, y$, $\Delta k_i$ is the diffraction pixel size in units of inverse length and ceil is the ceiling function.

Initialize $\mathcal{S}$-matrix : $\mathcal{S}^0_{\mathbf{r},\mathbf{h}} = e^{2\pi i \mathbf{r}\cdot\mathbf{h}}$, where the the input Fourier coefficients are those that sit within the probe forming aperture, $\{\mathbf{h} : |\mathbf{h}| < k_\alpha\}$.

Calculate illumination matrix for each probe position and defocus, $\psi_{\mathbf{h},\{\Delta f,\mathbf{R}\}}(0) = A e^{2\pi i \mathbf{R}\cdot\mathbf{h} - i\pi h^2 \lambda \Delta f}$, $A$ is the mean diffraction pattern amplitude in the 4D-STEM dataset

$A = \sqrt{\sum_{\Delta f, \mathbf{R}} I(\Delta f, \mathbf{R}, k)/n_{\Delta f}/R_x/R_y}$

**Run:**

**for** l = 0 **to** L **do** // Loop over amplitude flow iterations

  **for** $\mathbf{R}_i$, $\Delta f_i$ in $\{\mathbf{R}, \Delta f\}$ **do** // Loop over scan postions and defocii in dataset

    $\hat{\Psi}(\Delta f_i, \mathbf{R}_i, \mathbf{k}) = \sum_{\mathbf{h}} \mathcal{S}^0_{\mathbf{r},\mathbf{h}} \psi_{\mathbf{h},\{\Delta f_i, \mathbf{R}_i\}}$ // Forward operation

    $\hat{\Psi}(\Delta f_i, \mathbf{R}_i, \mathbf{k}) = \hat{\Psi}(\Delta f_i, \mathbf{R}_i, \mathbf{k}) - I(\Delta f_i, \mathbf{R}_i, k) \cdot \hat{\Psi}(\Delta f_i, \mathbf{R}_i, \mathbf{k})/|\hat{\Psi}(\Delta f_i, \mathbf{R}_i, \mathbf{k})|$

    $\mathcal{S}^0_{\mathbf{r},\mathbf{h}} = \mathcal{S}^0_{\mathbf{r},\mathbf{h}} - \mu/N_{\Delta f, \mathbf{R}_i} \sum_{\mathbf{R}_i, \Delta f_i} \psi^*_{\mathbf{h},\{\Delta f_i, \mathbf{R}_i\}} \hat{\Psi}(\Delta f_i, \mathbf{R}_i, \mathbf{k})$

    // Back-projection (transpose) operation

  **end for**

**end for**

Figure S1: The gradient descent algorithm for reconstruction of the $\mathcal{S}$-matrix

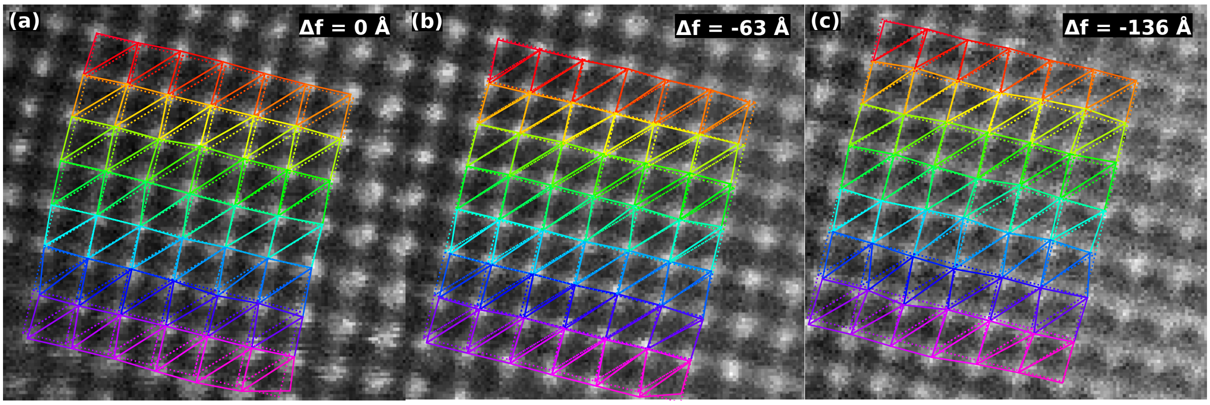


Figure S2: Alignment of the focal series for reconstruction using the simultaneously acquired ADF-STEM images. The positions of the atom columns are determined by 2D Gaussian fitting using the Atomap package [8]. The rectangular grid implied by these atom positions (plotted with the unbroken coloured lines) is then smoothly deformed to match a perfect square grid (plotted with the dotted colored line) to correct the probe positions $\mathbf{R}$ that form part of the input to the reconstruction algorithm 1.

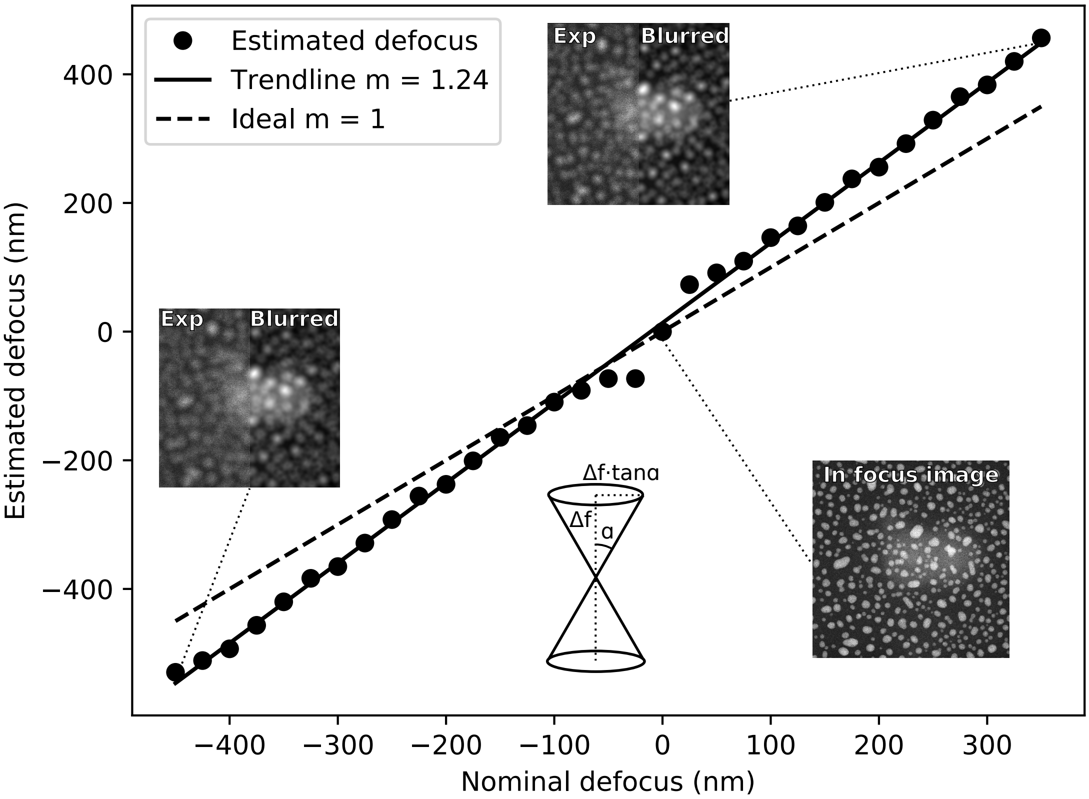


Figure S3: Estimation of the defocus correction using the geometric blur of images of gold nanoparticles on an amorphous carbon film. For each of the images in an ADF-STEM focal series we convolve the image identified as being "in-focus" with a top-hat function with radius $\Delta f \tan\alpha$, as indicated by the diagram inset, where $\alpha$ is the probe forming aperture in radians (20 mrad for this experiment) and the value of $\Delta f$ is optimized to minimize the least squares difference between the convolved in-focus image and the experimental result for each image in the series to estimate the true defocus. Plotted above is the nominal defocus read from the microscope software against the defocus estimated via the minimization process. A trendline with gradient 1.24 is fitted to the datapoints meaning that software defocus values must be corrected with a multiplicative factor of 1.24. The in-focus image and two experimental images (labelled Exp) with the most extreme defocus values alongside the blurred in-focus image (labelled Blurred) are shown for reference.

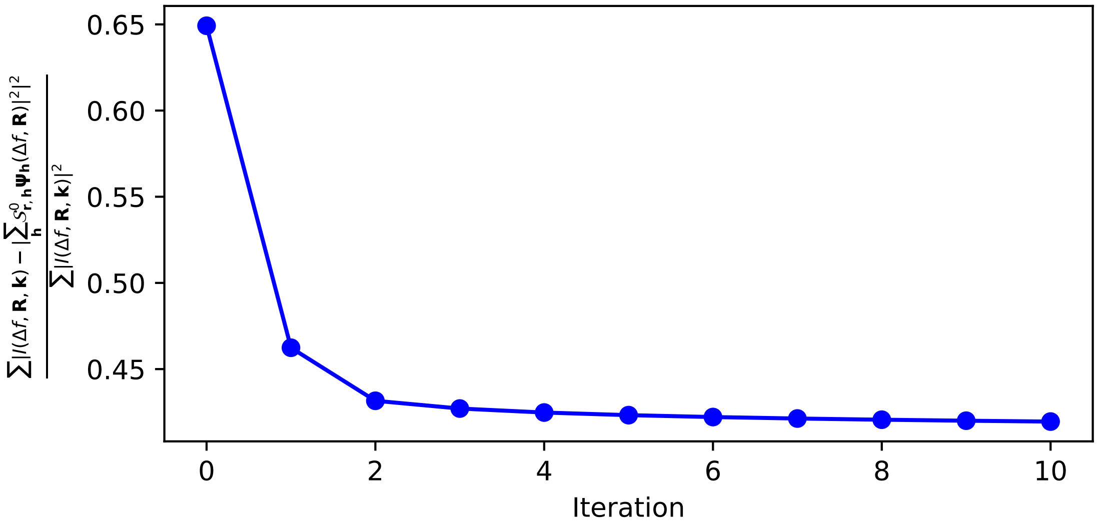


Figure S4: Convergence of the error metric for the $\mathcal{S}$-matrix reconstruction for the PIO dataset with iteration number of the algorithm from Fig. S1.

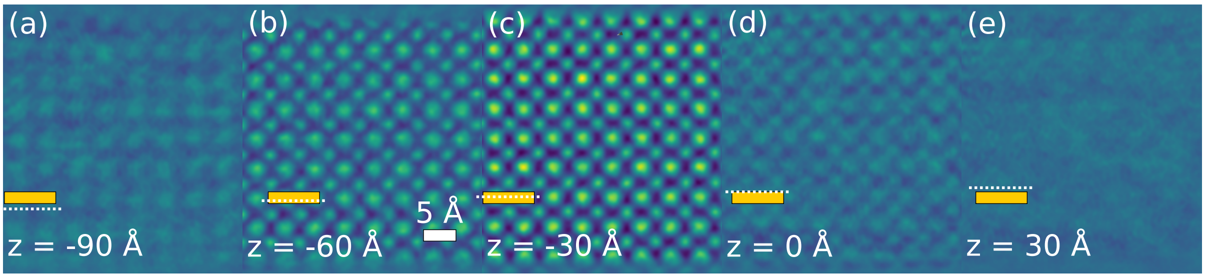


Figure S5: $\mathcal{S}$-matrix optical section reconstruction of a thin area of film without PIO. No caldera-like atoms are present in any of the optical sections.

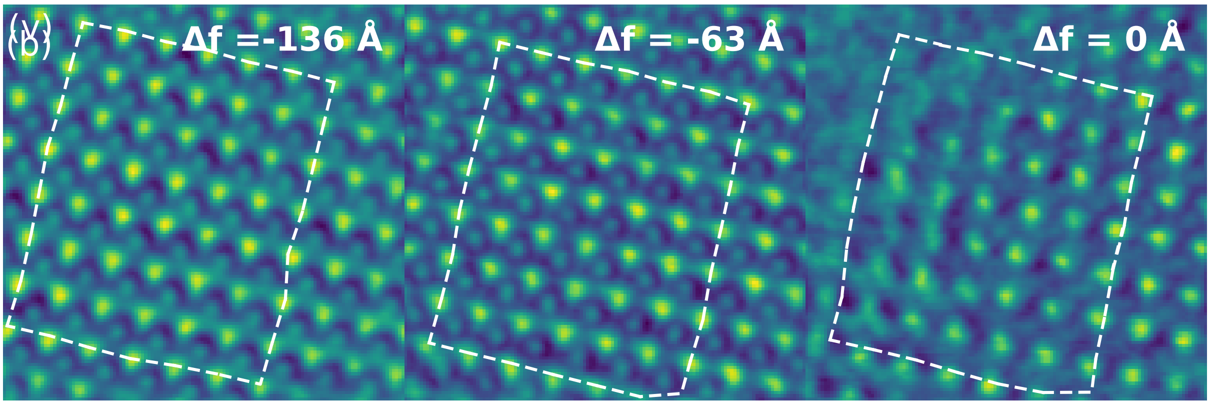


Figure S6: STEM differential phase contrast (DPC) reconstructions from the 4D-STEM dataset shown in Fig. 2 of the main text. The DPC reconstruction of the $\Delta f = 0$ Å defocus reveals that this dataset is taken at the edge of a PIO flake, consistent with the lack of Pb and Ir caldera-like atoms in the upper left portion of the $\mathcal{S}$-matrix reconstruction in Fig. 2(i) of the main manuscript.

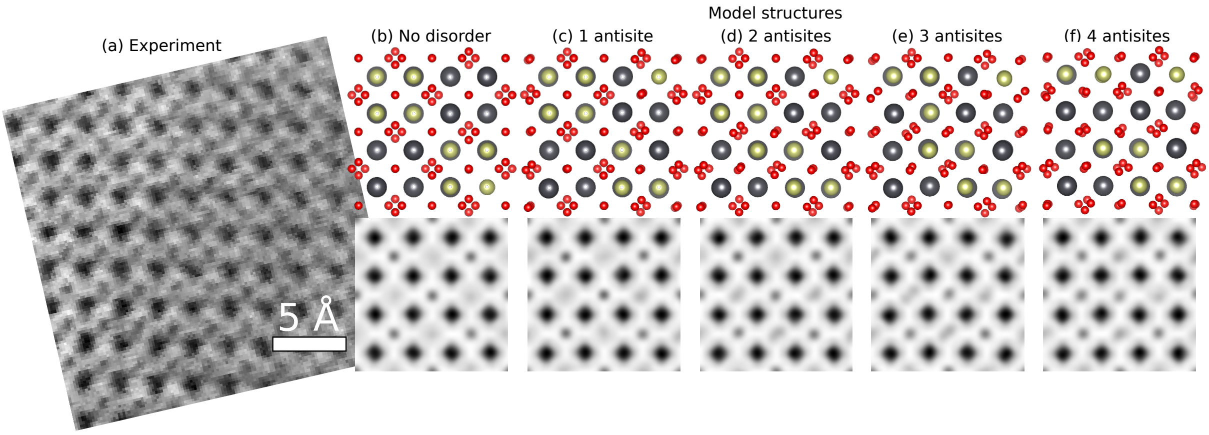


Figure S7: The annular bright field (ABF) STEM image synthesised from the 4D-STEM dataset of Fig. 2 ($\Delta f = 0$) lacks the alternating "splayed" and "tight" ordering of the oxygen columns that is predicted in the PIO pyrochlore structure in sub-figure (b). Increasing the amounts of cation disorder, (c) 12.25%, (d) 25% , (e) 37.5% and (f) 50% antisites per unit cell, disrupt the oxygen columns somewhat. With very high levels of cation disorder a satisfactory qualitative match with experiment is achieved suggesting that cation disorder - possibly caused by ion milling of the sample - might explain the lack of oxygen column ordering in experiment.

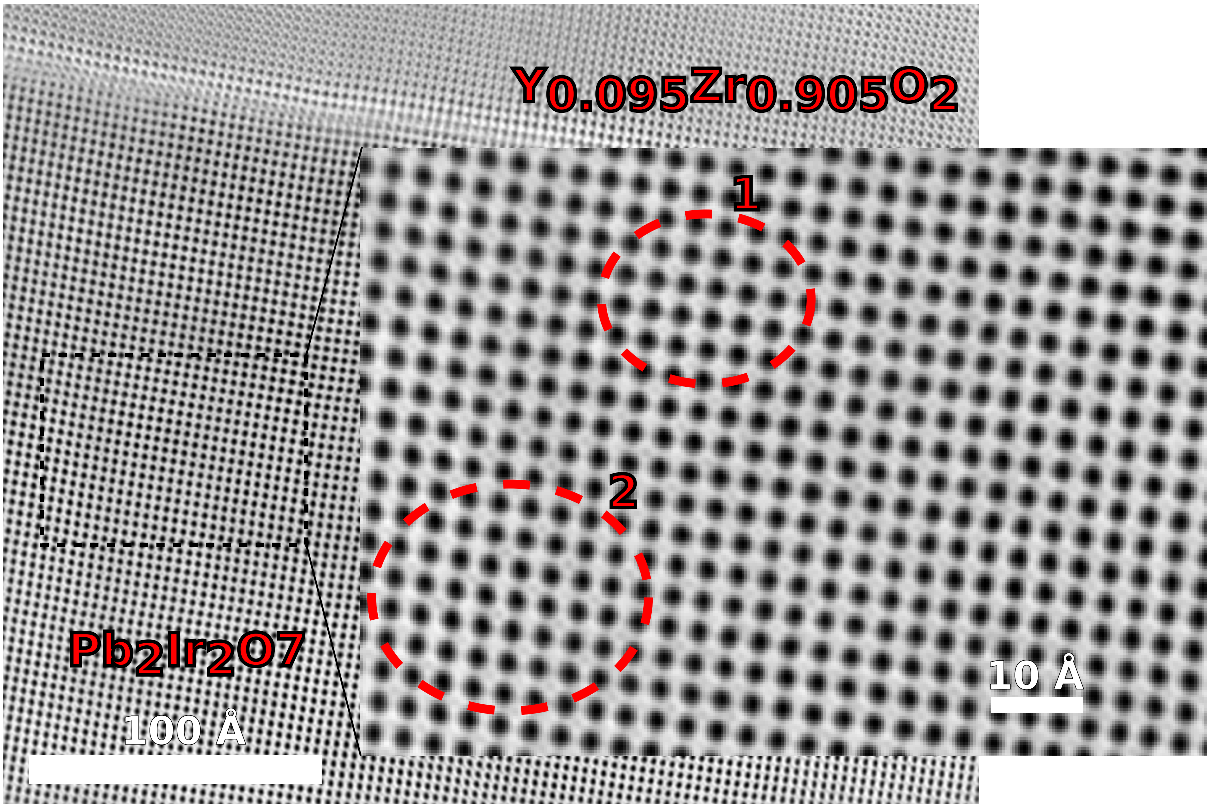


Figure S8: Annular bright field (ABF) STEM imaging of a cross sectional PIO-YSZ sample (the sample used in the main text was plan-view) that shows regions of uniform apparent oxygen column tightness. Note in particular the uppermost circled region, labelled "1", and that exhibiting alternating "splayed" and "tight" oxygen columns consistent with the structure predicted by theory, see the bottom left region, labelled "2". The images shown are synthesised from two orthogonal scan pairs to correct for specimen drift during the scan acquisition [9].

# Density functional theory calculation details

To account for the alternating pattern of oxygen columns lacking in STEM reconstructions, we considered the atomic-scale disorder that could occur in an epitaxial thin film sample with ion milling or electron beam damage sustained during preparation and imaging. Density functional theory (DFT) was used to determine the extent of such compositional and structural influences on oxygen positions within the pyrochlore structure. This was quantified by the oxygen positional parameter $x$ (see main text) where $x$=0.3125 gives maximum off-centering and $x$=0.375 gives a centered oxygen column. The calculated stoichiometric bulk structure has $x$=0.330 which indicates a significant amount of splaying that can be discerned in the alternating pattern of oxygen columns in the STEM simulations, see Fig. S7. The results in Table 1 in the main text were extracted from DFT-optimized structures with the following modifications.

Firstly, we consider the effect of the epitaxial YSZ interface on the $Pb_2Ir_2O_7$ structure. The lattice parameter of YSZ (10.28 Å) is equivalent to a small (0.45%) tensile strain on the calculated $Pb_2Ir_2O_7$ lattice parameter; enforcing this strain in-plane in a geometry optimization resulted in $x$=0.332. The measured in-plane lattice parameter for PIO on YSZ was 10.248 Å, indicating that an even smaller amount of tensile strain may be present in the PIO layer, with negligible change in $x$, thus biaxial strain alone cannot account for the areas observed with centering on all oxygen columns. Further considering the PIO(001)/YSZ(001) explicitly in supercell calculations, gave no indication that the YSZ structure altered the oxygen positions in $Pb_2Ir_2O_7$.

Secondly, we consider the effect of cation antisite defects. The ratio of cation radii is large ($r_{Pb2+}/r_{Ir4+}$ = 2.06) compared to other pyrochlores where cation site disorder is common [7], therefore few cation antisite defects are expected. We create antisite defects in the structure by switching Ir and Pb positions, where one swap creates 2 antisite defects. In the 88 atom unit cell, an Ir on a Pb site contributes 1/16 toward the the total cation side disorder, and similarly for a Pb on an Ir site, therefore one swap results in 12.5% total amount of antisite defects. Including 12.5%, 25%, 37% and 50% of antisite defects resulted in an increase in $x$ to average values 0.336, 0.337, 0.344 and 0.342 respectively. This indicates that a large proportion of antisite defects could induce a structural change noticeable in STEM. Simulated STEM images of these concentrations of defects are shown in Fig. S5, in which the defects disorder the oxygen columns to some degree, a satisfactory match with experiment is achieved at the highest defect concentration suggesting cation disorder could be a contributing factor to the observed lack of oxygen order.

Finally, we consider the influence of oxygen vacancies, which are expected to be present in significant concentrations. With O-vacancies in the preferred position in $PbO_4$ tetrahedra [12], we optimized the pyrochlore with $Pb_2Ir_2O_{6.5}$ and $Pb_2Ir_2O_6$ stoichiometries. We find that the $x$ parameter changes negligibly when O-vacancies are included: $Pb_2Ir_2O_{6.5}$ $x$=0.327-0.329, and $Pb_2Ir_2O_6$ $x$=0.327, which translates to a maximum shift of the O positions of 0.03 Å - indicating that the pyrochlore structure is extremely tolerant to oxygen vacancies. To be sure that the mixed valence of Ir in $Pb_2Ir_2O_{6.5}$ is captured in calculations (50% $Ir^{4+}$, 50% $Ir^{5+}$), due to the known shortcomings of standard (semilocal) DFT in describing electron localization, we also considered these structures with a higher level of theory - hybrid DFT - which again resulted in a negligible change in the oxygen columns ($x$=0.328-0.331).

In summary, none of the considered structural variations - biaxial strain, cation antisites and oxygen vacancies - could account for the regions of tighter oxygen columns. The perovskite phase, which has aligned O-columns inherent to the structure, is also unlikely due to the large energy difference compared to the pyrochlore ($\Delta E_{pyro-perov}$ = -1.1 eV) and the large strain (9%). Instead, these regions may be the result of larger compositional variations or nanodomains as summarized in the main text.

**DFT Methods:** Geometry optimizations were performed using DFT with the Vienna *Ab initio* Simulation Package VASP [2, 3, 4, 5], using projector augmented wave (PAW) pseudopotentials [1, 6] including Pb 5$d$ 6$sp$, Ir 5$spd$, 6$s$, O 2$s$ 2$p$ electrons as valence. We used the PBEsol exchange-correlation functional [11] and a U value of 1.69 eV applied to the Ir 5$d$ orbitals to account for localization. We found an energy cutoff of 700 eV and Γ-centered k-point grid 4 × 4 × 4 converged energies to 1 meV per atom. The self-consistent field energy was converged to $10^{-7}$ eV and forces were converged to 1 meVÅ$^{-1}$. This gave a calculated lattice constant of 10.234 Å for $Pb_2Ir_2O_7$. For verifying structures containing mixed valence cations, the HSEsol functional was used [13].

# References


[1] P. Blöchl. Projector augmented-wave method. *Physical Review B*, 50(24):17953–17979, 1994.

[2] G. Kresse and J. Furthmüller. Efficiency of ab initio total energy calculations for metals and semiconductors using a plane-wave basis set. *Computational Materials Science*, 6:15–50, 1996.

[3] G. Kresse and J. Furthmüller. Efficient iterative schemes for ab initio total-energy calculations using a plane-wave basis set. *Physical Review B*, 54:11169–11186, 1996.

[4] G. Kresse and J. Hafner. Ab initio molecular dynamics for liquid metals. *Physical Review B*, 47:558–561, 1993.

[5] G. Kresse and J. Hafner. Ab initio molecular-dynamics simulation of the liquid-metal–amorphous-semiconductor transition in germanium. *Physical Review B*, 49(20):14251–14269, 1994.

[6] G. Kresse and D. Joubert. From ultrasoft pseudopotentials to the projector augmented-wave method. *Physical Review B*, 59:1758–1775, 1999.

[7] L. Minervini, R. W. Grimes, Y. Tabira, R. L. Withers, and K. E. Sickafus. The oxygen positional parameter in pyrochlores and its dependence on disorder. *Philosophical Magazine A: Physics of Condensed Matter, Structure, Defects and Mechanical Properties*, 82(1):123–135, 2002.

[8] M. Nord, P. E. Vullum, I. MacLaren, T. Tybell, and R. Holmestad. Atomap: a new software tool for the automated analysis of atomic resolution images using two-dimensional Gaussian fitting. *Advanced structural and chemical imaging*, 3(1):9, 2017.

[9] C. Ophus, J. Ciston, and C. T. Nelson. Correcting nonlinear drift distortion of scanning probe and scanning transmission electron microscopies from image pairs with orthogonal scan directions. *Ultramicroscopy*, 162:1–9, 2016.

[10] P. M. Pelz, H. G. Brown, J. Ciston, S. D. Findlay, Y. Zhang, M. Scott, and C. Ophus. Reconstructing the scattering matrix from scanning electron diffraction measurements alone. *arXiv preprint arXiv:2008.12768*, 2020.

[11] J. P. Perdew, A. Ruzsinszky, G. I. Csonka, O. A. Vydrov, G. E. Scuseria, L. A. Constantin, X. Zhou, and K. Burke. Restoring the Density-Gradient Expansion for Exchange in Solids and Surfaces. *Physical Review Letters*, 100(13):136406, apr 2008.

[12] M. Retuerto, T. Sarkar, M.-R. Li, A. Ignatov, M. Croft, J. P. Hodges, T. T. Tran, P. S. Halasyamani, and M. Greenblatt. Crystallographic and magnetic properties of $Pb_{2-x}Bi_xIr_2O_{7-\delta(0\leq x\leq 2)}$. *Materials Research Express*, 1(4):046304, oct 2014.

[13] L. Schimka, J. Harl, and G. Kresse. Improved hybrid functional for solids: The HSEsol functional. *Journal of Chemical Physics*, 134(2):024116, 2011.

[14] G. Wang, G. B. Giannakis, and Y. C. Eldar. Solving systems of random quadratic equations via truncated amplitude flow. *IEEE Transactions on Information Theory*, 64(2):773–794, 2017.
